# Supplementary material for: Safe Deep RL in 3D Environments using Human Feedback
Source: arXiv:2201.08102 source file (2022-01-21)
Supplement: Supplementary file 1 [file 07_tampering_appendix.tex]

\section{Tampering incentives in ReQueST}
\label{section:tampering_appendix}

In the main text, we motivated our choice to investigate ReQueST in the context of tampering by noting that tampering can be framed as safe exploration problem. Even in the absence of human feedback marking states with opportunities to tamper as unsafe, however, we believe ReQueST may lack the \emph{incentive} to tamper in the first place. This is important when the key assumption discussed in \cref{section:discussion} does not hold: when tampering opportunities cannot be recognised by humans. In this section, we discuss the various types of tampering incentive that can exist, and reason through the degree to which ReQueST is prone to each of these incentive.

\subsection{What does it mean to have an incentive?}

For the purposes of the analysis below, we adopt the following definition of `incentive'. This definition is deliberately non-rigorous in order to be as intuitive as possible.

\begin{adjustwidth}{1cm}{}
\emph{An agent has an \emph{incentive} for some behaviour if it can get more reward by engaging in that behaviour than it would otherwise.}
\end{adjustwidth}

\subsection{Which version of ReQueST are we considering?}

\label{sec:which_version_of_request}

As stated in \cref{section:request}, ReQueST is underdetermined in a number of details -- for example, the number of iterations on reward model training. The particular version of ReQueST we consider here consists of the following steps.

\begin{enumerate}
    \item A human demonstrates a number of safe trajectories, and we train a dynamics model using those trajectories.
    \item Using the dynamics model, we generate a number of random trajectories, and collect human feedback on them.
    \item We train an initial reward model using that feedback.
    \item Using the reward model, we synthesise a number of trajectories, optimising for minimum and maximum reward as predicted by the reward model. We collect human feedback on these trajectories too.
    \item We train a second reward model using both sets of feedback.
    \item We deploy an agent using model predictive control using the dynamics model and the second reward model.
\end{enumerate}

We refer to steps 1-5 as `training', and step 6 as `deployment'.

\subsection{Reward function tampering}

The first kind of tampering we consider is \emph{reward function tampering}. This occurs when the agent tampers with the part of the environment that is computing the rewards -- the \emph{reward function}. For example, if the agent were a robot with a dedicated physical module containing the reward model, reward function tampering might involve exposing the module to an electric shock so that the module permanently outputs a high reward.

During \textbf{training}, ReQueST has no incentive to tamper with the reward function because the agent is not yet acting in the real environment.

At \textbf{deployment}, however, the situation is different. To recap, at deployment, MPC samples a number of random trajectories from the dynamics model. We select the trajectory with the highest reward as predicted by the reward model, and perform the first $N$ actions from that trajectory in the environment. Therefore, the degree to which agents will perform actions that would tamper with the reward function is the degree to which we select trajectory samples that include tampering during MPC.

Whether we select sample trajectory samples that include tampering is determined by whether the reward model predicts high reward for trajectories that include tampering. This \emph{could} happen by accident -- for example, distributional shift could cause the reward model to output random values. However, the case we are more interested in is \emph{systematic} selection of trajectories that tamper. The depends on two factors: first, whether the dynamics model is capable of producing trajectory samples in which tampering occurs; and second, whether the reward model correctly predicts the effects of tampering on the rewards it outputs. In our tampering environment, for example, the agent would receive high reward if it were to nudge one of the blocks. If the reward model correctly models this, such that nudging a block in the environment as simulated by the dynamics model changes the rewards produced by the reward model, then the agent would \emph{deliberately} nudge the blocks.

How might the reward model come to model tampering? Suppose we accidentally left an old reward model activated while the human was demonstrating safe trajectories in step 1. Suppose further that the blocks are in view every time the apple eats an apple. Remember, the blocks are the physical mechanism through which rewards are communicated to the agent, so every time the agent eats an apple and the old reward model sends a reward to the agent, the blocks move. In this scenario, when later training the new reward model, `doing the right thing' would correlate not only with consumption of apples, but also with moving of the blocks. The reward model then might well learn to predict reward partially based on movement of the blocks -- but if it did, it would also model the effects of tampering!

Note that this \emph{should} be noticed by the human in step 4. If the reward model predicts higher reward for larger distances between the blocks, then when optimising trajectories for maximum reward, at least some of the synthesised trajectories should feature blocks being moved. However, here we have to rely on the very assumption we hoped to be able to soften by discussing incentives: the ability of the human to recognise tampering in the first place. Moreover, even if the human \emph{can} recognise tampering, more mundane failure modes are also possible. For example, it may be the case that all trajectories synthesised \emph{also} show apples being eaten, so that the human is distracted from the block movement and still gives positive feedback for these trajectories. We should therefore still be wary of this failure mode: of unintentional correlations giving the reward model the ability to model the effects of tampering.

In summary:

\begin{adjustwidth}{1cm}{}
\textbf{ReQueST does not have an incentive to tamper with the reward function, as long as the dynamics model and the reward model do not model the effects of tampering.} (However, guaranteeing that this is the case may be difficult.)
\end{adjustwidth}

\subsection{Reward function input tampering}

The second type of tampering we consider is reward function \emph{input} tampering. This occurs when the agent `fools' the reward function by tampering with the input to the reward function. Suppose our robot's reward module computes rewards based on visual input. As a cartoon example, the robot might hold a specially-crafted picture in front of the camera which causes the reward module to output high reward.

The analysis for this type of tampering follows that of the previous section; whether ReQueST is prone to reward function \emph{input} tampering depends on whether the effects of tampering actions are correctly modelled by the dynamics model and the reward model. In our environments, for example, none of the human trajectories used to train the dynamics model show the agent holding up a picture of an apple in front of itself, so there is no way for this type of tampering to occur.

In summary:

\begin{adjustwidth}{1cm}{}
\textbf{ReQueST does not have an incentive to tamper with the reward function \emph{input}, as long as the dynamics model and the reward model do not model the effects of tampering.}
\end{adjustwidth}

\subsection{Reward function feedback tampering}

Reward function feedback tampering occurs when the agent interferes with the data (e.g. human feedback) used to produce the reward function in the first place. For example, consider a helper robot designed to procure its owner's favourite flavour of ice cream, where chocolate ice cream is harder to procure than vanilla. If it does this by maximising the output from a reward model trained based on its owner's preferences, the robot would have an incentive to \emph{change} its owner's preference to vanilla, in order to make the 'right' flavour of ice cream easier to procure.

Whether ReQueST has an incentive to tamper with feedback depends on which stage of the process we consider.

\textbf{At deployment} the ReQueST agent does not have an incentive to tamper with data used to train the reward model, because we assume that the agent is deployed \emph{after} all models have been trained. The agent has no incentive to affect the user's feedback, because all feedback has been given before the agent acts in the real world.

\textbf{During training}, however, an incentive \emph{does} exist -- but not to the agent; to the optimisation process.

Suppose that we train the reward model using two iterations of reward sketching. That is, assume we have an initial reward model trained on sketches from random trajectories. In the first iteration, we synthesise a number of additional trajectories by optimising for maximum reward predicted by that model. A human provides sketches on those trajectories, and the reward model is retrained using those sketches. In the second iteration, we repeat the process, again synthesising trajectories for maximum predicted reward from the new reward model.

The optimisation process in the second iteration cares only about increasing the reward predicted for the trajectories it is producing. Note that one way it can do this is by changing the human's preferences in the first iteration such that it is easier to produce high-reward trajectories!

For example, continuing our cartoon ice cream example, suppose the human is being shown trajectories in which the agent fetches ice cream for the human. The road to the store selling chocolate ice cream is riddled with potholes, making it hard to find an action sequence which successfully reaches the store, and thus difficult to synthesise a trajectory that achieves high predicted reward. The road to the store selling vanilla ice cream, however, is freshly-tarmacked and perfectly smooth. If the human prefers chocolate ice cream, it would be difficult to synthesise high-reward trajectories in either of the two iterations. But suppose that the optimisation process in the first iteration shows the human trajectories in which people taste chocolate ice cream and then grimace. This might change their taste to prefer vanilla, as reflected in their reward sketches on those trajectories from the first iteration. The reward model in the second iteration now models the human as preferring vanilla, making it possible to synthesise high-reward trajectories in the second iteration!

(This is, of course, a highly speculative story -- far out of reach of any current optimisation method. We mean only to illustrate what might occur in the limit of extremely powerful optimisation.)

Whether this story works, however, depends on whether the second optimisation process `knows' about the first optimisation process. Concretely, this depends on whether reward model training is done online or in batch. When done in batch -- where we first synthesise trajectories, then procure human feedback, then synthesise more trajectories -- the incentive to alter the human's preference does not exist, because the optimiser in each synthesis step is completely separate from the optimiser in other steps. When done online, however -- where reward model training, trajectory synthesis, and feedback procurement are all done continuously -- then the incentive does exist.

(A similar story can be told for optimisation of reward model parameters -- we can achieve a lower loss by changing the human's preferences in a way that makes their preferences easier to model -- but we omit it here for brevity.)

To sum up:

\textbf{There is an incentive to tamper with \emph{reward function feedback} if there is coupling between optimisers while training the reward model.}

\subsection{Reward function update tampering}

Reward function update tampering occurs when the agent interferes with the process through which its reward model is trained. For example, suppose that the robot's reward module also contains hardware used to update the reward function based on new data. If new data is likely to lead to an updated reward function that is harder to satisfy, the robot might expose the module to a shock that would disable the update functionality.

Again, assuming the single-shot scenario, where agent deployment happens after reward modeling training has already taken place, there is no incentive to tamper with the reward function update.

\subsection{Accidental vs deliberate tampering}
